# Supplementary material for: DV-Lens: Revealing the Functional Organization of Language Model Parameters
Source: arXiv:2610.04489 source file (2026-11-18)
Supplement: Supplementary file 1 [file supp_style.tex]

\usepackage{etoc}
\usepackage{multicol}
\makeatletter
\renewcommand\extCounters[4]{\setcounter{figure}{#1}\setcounter{table}{#2}%
  \setcounter{equation}{#3}\@ifundefined{c@algorithm}{}{\setcounter{algorithm}{#4}}}
\makeatother
\colorlet{suppaccentlight}{suppaccent!12}
\colorlet{supprule}{suppaccent!45}

\makeatletter
\setcounter{tocdepth}{2}
\newlength{\suppSecNum}\setlength{\suppSecNum}{1.55em}
\newlength{\suppSubNum}\setlength{\suppSubNum}{2.15em}
\newlength{\suppPage}\setlength{\suppPage}{1.9em}
\etocsettocstyle{}{}
\etocsetstyle{section}{}
  {\par\addvspace{4.5pt}}
  {\noindent\leftskip\z@\hangindent\suppSecNum\rightskip\glueexpr\suppPage+0pt plus 4em\relax\parfillskip-\suppPage\relax
   \makebox[\suppSecNum][l]{\textcolor{suppaccent}{\bfseries\etocthenumber}}%
   {\bfseries\etocname}\nobreak\hfill\nobreak
   \makebox[\suppPage][r]{\textcolor{suppaccent}{\bfseries\etocthepage}}\par\nopagebreak}
  {}
\etocsetstyle{subsection}{}
  {\par\addvspace{0.6pt}}
  {\noindent\leftskip\suppSecNum\hangindent\suppSubNum\rightskip\glueexpr\suppPage+0pt plus 4em\relax\parfillskip-\suppPage\relax
   \makebox[\suppSubNum][l]{\etocnumber}\etocname\nobreak
   \leaders\hbox to 0.55em{\hss\textcolor{supprule}{.}\hss}\hfill\nobreak
   \makebox[\suppPage][r]{\etocpage}\par}
  {}
\makeatother
\makeatletter
\newcommand{\suppFrontMatter}{%
  \onecolumn
\setlength{\columnsep}{1.6em}
\setlength{\columnseprule}{0.4pt}
\renewcommand{\columnseprulecolor}{\color{supprule}}


  \begin{center}
    {\Large\bfseries\thetitle\par}
    \vspace{0.45em}
    {\large Appendix\par}
  \end{center}
  \vspace{0.5em}
  \noindent{\color{suppaccent}\rule{\linewidth}{0.9pt}}\par\nobreak
  \vspace{3pt}
  \noindent\colorbox{suppaccentlight}{\makebox[\dimexpr\linewidth-2\fboxsep\relax][l]{%
    \textcolor{suppaccent}{\large\bfseries Contents}}}\par\nobreak
  \vspace{4pt}
  \begingroup\small\hypersetup{linkcolor=black}%
  \raggedcolumns\interlinepenalty\@M%
  \begin{multicols}{2}
    \etocsettagdepth{main}{none}\etocsettagdepth{appendix}{subsection}\tableofcontents
  \end{multicols}
  \endgroup
  \vspace{2pt}
  \noindent{\color{suppaccent}\rule{\linewidth}{0.9pt}}\par
  \vspace{6pt}}
\makeatother
